# Supplementary material for: Identifying efficient controls of complex interaction networks using genetic algorithms
Source: arXiv:2007.04853 ancillary file (2020-07-09)
Supplement: Supplementary file 1 [file supplementary-material.pdf]

# Supplementary Material

## 1 Data

The data analyzed in the article is provided as supplementary information in two ZIP archives. The obtained results are shown in an Microsoft Excel workbook.

### 1.1 Input

The *Input* archive contains the input data that was analyzed in the article. The actual networks can be found in the text files named *Network\_Name*. Each network file has a corresponding target nodes file named *Network\_Name.Target*. Both such files are needed for one run of the application. Furthermore, the files corresponding to the protein-protein interaction networks have an additional drug-target nodes file named *Network\_Name.Preferred*, which can be used as supplementary input.

### 1.2 Output

The *Output* archive contains the results obtained after running the application once on each of the networks in the *Input* directory. Each output consists of a JSON file named *Network\_Name.Output*. In addition, the application has been run once more for all the protein-protein interaction networks while using the additional preferred nodes. The files named *Network\_Name.Preferred.Output* contain these results.

Given the stochastic nature of the algorithm, the results obtained after each run of the application might vary. Each file represents only one possible output.

### 1.3 Results

The *Results* file contains an overview of the results obtained after analyzing each of the networks in the *Input* directory using the algorithm presented in the article, as well as a comparison on the results obtained by two other similar algorithms on the same sets of input data.

## 2 Software

The algorithm has been implemented as a C# / .Net Core application. The application is cross-platform, working on all modern operating systems (Windows, MacOS, Linux), and can be run through a web-based GUI (graphical user interface), or via CLI (command-line interface).

### 2.1 Download

You can either download the repository or the already compiled application.

#### 2.1.1 Build

The repository consists of a Visual Studio 2019 project. You can download it to run or build the application yourself. You need to have .NET Core 3.1 [1] installed on your computer in order to run it, or the corresponding SDK in order to also be able to build it.

#### 2.1.2 Release

You can directly download the application (corresponding to your operating system) from the GitHub repository [2]. No prerequisites are needed in order to run it, although permission to execute the application and permission to create files might be required.

After downloading the ZIP archive, simply unarchive it and it is ready to run, without any installation. Please note that on MacOS and Linux it might be needed to manually mark the file “GeneticAlgNetControl” as executable.

### 2.2 Usage

Some options (such as CLI) require adding several command-line arguments when launching the application. This can be achieved by launching the application from your operating system’s terminal or console. In order to find out more about the usage and possible arguments which can be used, you can launch the application with the `--Mode` argument set to *Help*.

#### 2.2.1 GUI

To run the application via GUI, it is enough to double click the “GeneticAlgNetControl” file or launch it from the terminal either with no arguments (default), or with the `--Mode` argument set to *Web*. This mode has one optional argument:

1. `--Urls`. (optional) Use this argument to specify the local address on which to run the web server. It can also be configured in the “appsettings.json” file. The default value is “http://localhost:5000”.

Logging is enabled by default, so you will get several information messages throughout the execution of the application, firstly notifying that a local web server was started on your computer. If there is another local server that uses “localhost” on the default ports 5000 and 5001, the application may encounter an error and fail to start. You can change the ports that are used by launching the application with the `--Urls` argument.

Your default browser should open automatically to the home page of the application. If not, you should copy the local web server’s address and paste it into the address bar of your favorite browser. Afterwards, it can be used just as any other website / web application (with the difference that everything runs locally, so no internet connection is needed). The application was tested on Chrome, but it should render and work nicely in any browser.

If the “https” protocol is used (so, requesting a secure connection), your browser might issue a warning that the certificate of the website could not be verified, thus the connection might not be secure. Considering that everything happens locally (the web server is hosted on your computer, and the browser connects locally to it), no certificate is actually needed, as no data gets transferred, and the warning can be safely ignored (by selecting the options similar to “I understand the risks.” or “I want to continue anyway.”).

To close the application, you can navigate to the “Quit” page, or you can simply select the terminal where the application is running (and not the browser!) and press `CTRL+C` (or `CMD+C` on MacOS). It is recommended to wait for it to gracefully shut down, as this will automatically stop and save the progress of all currently running analyses. If you forcefully close the application, you will lose all progress on the currently running analyses, however they will automatically restart on the next application launch.

### 2.2.2 CLI

To run the application via CLI, you need to launch it from the terminal with the `--Mode` argument set to `Cli`. This mode has three mandatory arguments (omitting any of them will return an error) and two optional ones:

1. `--Edges`. Use this argument to specify the path to the file containing the edges of the network. Each edge should be on a new line, with its source and target nodes being separated by a semicolon character, for example:

```
Node A;Node B
Node A;Node C
Node A;Node D
Node C;Node D
```

If the file is in a different format, or no nodes or edges could be found, an error will be returned. The order of the nodes is important, as the network is directed. Thus, “Node A;Node B” is not the same as “Node B;Node A”, and they can both appear in the network. Any duplicate edges will be

ignored. The set of nodes in the network will be automatically inferred from the set of edges. This argument does not have a default value.

2. – – *Targets*. Use this argument to specify the path to the file containing the target nodes of the network. Each node should be on a new line.

```
Node C
Node D
```

If the file is in a different format, or no nodes could be found in the network, an error will be returned. Only the nodes which already appear in the network will be considered. Any duplicate nodes will be ignored. This argument does not have a default value.

3. – – *Preferred*. (optional) Use this argument to specify the path to the file containing the preferred nodes of the network. Each node should be on a new line.

```
Node A
Node C
```

If the file is in a different format, or no nodes could be found in the network, an error will be returned. Only the nodes which already appear in the network will be considered. Any duplicate nodes will be ignored. This argument does not have a default value.

4. – – *Parameters*. Use this argument to specify the path to the file containing the parameter values for the analysis. The file should be in JSON format, using the same model as the “DefaultParameters.json” file, which contains the default parameter values.

```
{
  "RandomSeed": -1,
  "MaximumIterations": 10000,
  "MaximumIterationsWithoutImprovement": 1000,
  "MaximumPathLength": 5,
  "PopulationSize": 80,
  "RandomGenesPerChromosome": 15,
  "PercentageRandom": 0.25,
  "PercentageElite": 0.25,
  "ProbabilityMutation": 0.01,
  "CrossoverType": 0,
  "MutationType": 0
}
```

The parameters are presented below.

- (a) *RandomSeed*. Represents the random seed for the current algorithm run. It must be a positive integer. However, if it is  $-1$ , then it will be randomly generated. Its default value is  $-1$ , which means that it will be randomly generated every time.
- (b) *MaximumIterations*. Represents the total number of generations for which the algorithm will run. It must be a positive integer, and its default value is 10000.
- (c) *MaximumIterationsWithoutImprovement*. Represents the total number of generations without an improvement in the fitness of the best chromosome in the population. It must be a positive integer, and its default value is 1000.
- (d) *MaximumPathLength*. Represents the maximum number of edges in a control path. It must be a positive integer, and its default value is 5.
- (e) *PopulationSize*. Represents the total number of chromosomes in a generation. It must be a positive integer greater than 1, and its default value is 80.
- (f) *RandomGenesPerChromosome*. Represents the maximum number of randomly generated genes in a chromosome. It must be a positive integer, and its default value is 15.
- (g) *PercentageElite*. Represents the maximum percentage of elite chromosomes in a generation. It must be a real number in the  $[0, 1]$  interval, and its default value is 0.25.
- (h) *PercentageRandom*. Represents the maximum percentage of randomly generated chromosomes in a generation. It must be a real number in the  $[0, 1]$  interval, and its default value is 0.25.
- (i) *ProbabilityMutation*. Represents the probability of mutation for a chromosome. It must be a real number in the  $[0, 1]$  interval, and its default value is 0.01.
- (j) *CrossoverType*. Represents the crossover algorithm to be used by the genetic algorithm. It must be an integer in the set 0, 1, 2, 3, and its default value is 0.
- (k) *MutationType*. Represents the mutation algorithm to be used by the genetic algorithm. It must be an integer in the set 0, 1, 2, 3, and its default value is 0.

If the file is in a different format, an error will be returned. Additionally, if any of the parameters are missing, their default values will be used. This argument does not have a default value.

- 5. *--Output*. (optional) Use this argument to specify the path to the output file where the solutions of the analysis will be written. Permission to write is needed for the corresponding folder. If a file with the same name already

exists, it will be automatically overwritten. The default value is the name of the file containing the edges, followed by the current date and time.

If all the files have been successfully read and loaded, a confirmation message will be logged to the terminal and the algorithm will start running, providing constant feedback on its progress. Upon completion, all of the solutions will be written to the JSON file specified by the `--Output` argument.

## References

- [1] Microsoft. .net core, 2019. Available at <https://dotnet.microsoft.com/>, version 3.1.
- [2] Victor Popescu. Geneticalgnetcontrol, 2020. Available at <https://github.com/vicbgdn/GeneticAlgNetControl>, version 1.0.
